# Supplementary material for: WARPD: World model Assisted Reactive Policy Diffusion
Source: arXiv:2410.14040 source file (2025-12-12)
Supplement: Supplementary file 1 [file SI.tex]

\subsection{Societal Impact}
\label{app:societal_impact}
This paper presents work intending to advance the field of Machine Learning in Robotics. 
The authors are committed to ensuring that the research is used for the benefit of society and does not contribute to any harm or negative consequences.
While there are many potential societal consequences robotics and machine learning in general, there are none that are specific to this work alone, that we can foresee.
